# Supplementary material for: Thermoelectric properties of gapped bilayer graphene
Source: arXiv:1810.02280 ancillary file (2019-06-14)
Supplement: Supplementary file 1 [file suppinfo.pdf]

# Supplementary Information

## Thermoelectric properties of gapped bilayer graphene

Dominik Suszalski, Grzegorz Rut, and Adam Rycerz
*Marian Smoluchowski Institute of Physics, Jagiellonian University, Łojasiewicza 11, PL–30348 Kraków, Poland*
(Dated: June 15, 2019)

### I. DISPERSION RELATION, THE ACTUAL BANDGAP, AND DOPING

The Hamiltonian $H$ given by Eq. (4) in the main text leads to the dispersion relation for electrons [1]

$$E_{\pm}^{(e)}(\boldsymbol{k}) = \left[\frac{1}{2}t_{\perp}^2 + \frac{1}{4}U^2 + \hbar^2\left(v_F^2 + \frac{1}{2}v_3^2\right)k^2 \pm \sqrt{\Gamma(\boldsymbol{k})}\right]^{1/2},$$

$$\text{with}\ \ \Gamma(\boldsymbol{k}) = \frac{1}{4}\left(t_{\perp}^2 - \hbar^2 v_3^2 k^2\right)^2 + \hbar^2 v_F^2 k^2\left(t_{\perp}^2 + U^2 + \hbar^2 v_3^2 k^2\right) + 2\xi\, t_{\perp}\hbar^3 v_3 v_F^2 k^3 \cos 3\varphi, \tag{S1}$$

where $\pm$ refers to the upper/lower band, $\boldsymbol{k} \equiv (k_x, k_y)$ is the wavevector, with $\boldsymbol{k} = 0$ referring to the K or K' point (marked by $\xi = 1$ or $\xi = -1$, respectively), $k \equiv |\boldsymbol{k}|$, and the angle $0 \leqslant \varphi < 2\pi$ is the argument $\arg z$ of a complex number $z = k_x + ik_y$. For holes, we simply have $E_{\pm}^{(h)}(\boldsymbol{k}) = -E_{\pm}^{(e)}(\boldsymbol{k})$. This is a consequence of the combined particle-hole-reflection symmetry, which is preserved as we have neglected the next-nearest neighbor intralayer hopping ($t_2$). The precise value of $t_2$ ($\sim t_{\perp}$) is difficult to determine for BLG [2]; however, its effects are insignificant when discussing the band structure for $|E| \ll t_{\perp}$.

The value of a band gap $\Delta$ can be determined numerically via

$$\frac{\Delta}{2} = \min E_{-}^{(e)}(\boldsymbol{k}) = -\max E_{-}^{(h)}(\boldsymbol{k}). \tag{S2}$$

For $v_3 \neq 0$ the band gap can be approximated as follows

$$\Delta \approx \Delta_0\left(1 - \Delta_0\frac{\sqrt{2}v_3}{t_{\perp}v_F} - \Delta_0^2\frac{5v_3^2}{4U^2v_F^2}\right), \quad \text{with}\ \ \Delta_0 = \frac{|U|t_{\perp}}{\sqrt{U^2 + t_{\perp}^2}} \tag{S3}$$

($\Delta_0$ is the exact value of a gap in the absence of trigonal warping). Although its accuracy is better then 0.5% for $t' = 0.3\,\text{eV}$ and $|U| \leqslant 300\,\text{meV}$, the approximating Eq. (S3) is insufficient to present the numerical data in the energy scale used in Fig. 1(e) in the main text; instead, we have determined $\Delta$ for a given $U$ directly by performing the minimization in Eq. (S2) numerically.

In general, $\Delta < |U|$ for $|U| > 0$, leading to a peculiar (the Mexican hat-like) profile of the dispersion relation for $E_{-}^{(e)}(\boldsymbol{k})$ and $E_{-}^{(h)}(\boldsymbol{k})$ bands in the presence of a gap (see the second paper in Ref. [1]).

The dispersion relation given by Eq. (S1) also allows us to define the density of states at the Fermi energy ($E_F$) in a compact form

$$\rho(E_F) \equiv \rho^{(e)}(E_F) + \rho^{(h)}(E_F) = \frac{1}{\pi^2}\sum_{\substack{c=e,h\\ m=\pm}}\left|\frac{\partial}{\partial E}\,\mathcal{A}_m^{(c)}(E)\right|_{E=E_F}, \tag{S4}$$

where we took into account spin and valley degeneracies ($g_s = g_v = 2$) and $\mathcal{A}_{\pm}^{(e,h)}(E_F)$ denotes the area bounded by the Fermi surface in the $(k_x, k_y)$ plane. (In case $E = E_F$ is beyond the energy range of a given band, we put $\mathcal{A}_m^{(c)}(E) = 0$.) In particular, for $v_3 = 0$ and $\max(0, |E_F| - \Delta/2) \ll t_{\perp}$, we have

$$\rho(E_F) \approx \frac{t_{\perp}}{\pi(\hbar v_F)^2}\Theta\left(|E_F| - \Delta/2\right), \tag{S5}$$

with $\Theta(E)$ being the Heaviside step function. The prefactor in Eq. (S5) is often written in a form $2m_{\text{eff}}/(\pi^2\hbar)$, with the effective mass $m_{\text{eff}} \approx 0.033\,m_e$ (where $m_e$ is the free-electron mass) coinciding with the standard cyclotronic mass $m_C(E_F) = (\pi\hbar^2/2)\rho(E_F)$. Integrating Eq. (S5) over the energy, we obtain the physical carrier concentration (or *doping*) given by Eq. (5) in the main text.

At finite temperatures ($T > 0$), the *effective carrier concentration* can be defined via its relation to the Hall resistance, namely $R_H = -1/(en_{\rm eff})$ (with the electron charge $-e$), leading to

$$n_{\rm eff} = n_e - n_h = \int_0^\infty dE \rho(E) f_{\rm FD}(\mu, T, E) - \int_{-\infty}^0 dE \rho(E) \left[1 - f_{\rm FD}(\mu, T, E)\right], \tag{S6}$$

where $n_e$ ($n_h$) is the concentration of electrons (holes) and $f_{\rm FD}(\mu, T, E) = 1/\left[\exp\left((E-\mu)/k_B T\right) + 1\right]$ is the Fermi-Dirac distribution function for a given electrochemical potential $\mu$.

## II. TRANSMISSION PROBABILITY

### A. A semi-inifinite system in BLG

In the case of an abrupt potential barrier separating weakly- and heavily doped regions (see Fig. 1(a) in the main text) we start from the substitution in the Hamiltonian (see Eq. (4) in the main text) $\boldsymbol{p} \to \boldsymbol{p} + e\mathbf{A}$, with a vector potential $\mathbf{A} = (A_x, A_y)$ (not further specified, since it is disregarded in the forthcoming calculations). The $i$-th component of the current (with $i = x$ or $y$) corresponding to the Hamiltonian $H$ reads, for the $K$ valey,

$$j_i(\psi) = \psi^\dagger \cdot \left.\frac{\partial H}{\partial A_i}\right|_{A_i \to 0} \cdot \psi \quad \text{with} \quad \left.\frac{\partial H}{\partial A_i}\right|_{A_i \to 0} = e v_F \begin{pmatrix} 0 & 1 & 0 & 0 \\ 1 & 0 & 0 & \nu \\ 0 & 0 & 0 & 1 \\ 0 & \nu & 1 & 0 \end{pmatrix}, \tag{S7}$$

where we have defined a dimensionless parameter $\nu = v_3/v_F$.

Next, the transmission probability can be found by simple mode-matching of wavefunctions in the heavily- and weakly-doped regions. Although deriving the corresponding functions is not a challenging task, they cannot be presented in a closed form. Below, we briefly present a procedure for finding the solutions corresponding to waves moving in desired directions (i.e., to the left or to the right):

(i) The wavefunctions satisfying the Dirac equation $H\psi(x, y) = E\psi(x, y)$ can be found algebraically in to the momentum representation, $\pi_i = \hbar k_i$. The general solution has a form of a spinor $\psi(x, y) = \exp\left[i\left(k_x x + k_y y\right)\right] (\psi_1, \psi_2, \psi_3, \psi_4)^T$. There are four independent solutions, each corresponding to a different value of $k_x$ (for a system with periodic boundary conditions the transverse wave number $k_y = 2\pi n/W$, with $n = 0, \pm 1, \pm 2, ...$, and $W$ being the width of the system).

(ii) In order to determine the corresponding direction of propagation for a given solution of the Dirac equation, one needs to follow the subsequent two-step procedure. *First,* one has to check a sign of the current employing Eq. (S7). The positive (*or* negative) sign indicates the transmitted/incoming (*or* reflected) wave. *Second,* when dealing with the wavefunction carrying zero current, it is important to check the sign of the imaginary part of $k_x$. Positive (*or* negative) $\mathrm{Im}(k_x)$ corresponds to a solution decaying exponentially to the right (*or* to the left). When discussing the transmission through a single barrier separating the heavily- and weakly doped regions we can, however, limit ourselves to the solutions with real $k_x \neq 0$ (which are *normalizable* with respect to the carried current). Out of four solutions of the Dirac equation, there are at most two carrying a positive or negative current.

(iii) Subsequent calculation of the transmission probability becomes similar to the one usually performed for systems containing a sample area between two highly-conducting contacts. In the contact region, here modelled as heavily-doped bilayer graphene (for $x < 0$) the wavefunction takes a form

$$\psi_I(x) = \psi_{R,I}^{1(2)}(x) + r_1^{1(2)} \psi_{L,I}^1(x) + r_2^{1(2)} \psi_{L,I}^2(x), \tag{S8}$$

while the wavefunction in the weakly-doped sample area ($x > 0$) reads

$$\psi_{II}(x) = t_1^{1(2)} \psi_{R,II}^1(x) + t_2^{1(2)} \psi_{R,II}^2(x). \tag{S9}$$

The lower indexes, $R$ and $L$, refer to the waves moving to the right ($j_x > 0$) and to the left ($j_x < 0$), respectively. The upper indexes, 1(2), correspond to the two subbands. The parameters $r_1^{1(2)}$, $r_2^{1(2)}$, $t_1^{1(2)}$, $t_2^{1(2)}$ are closely related to the reflection and transmission probabilities and can be calculated via mode-matching at $x = 0$, namely: $\psi_I(0) = \psi_{II}(0)$. The final transmission probability is given by a sum over the all possible current ratios

$$T_{k_y} = \sum_{m,n} |t_n^m|^2 j_x\left(\psi_{R,II}^n\right) / j_x\left(\psi_{R,I}^m\right). \tag{S10}$$

The comparison of the Landauer-Büttiker conductance, following from Eq. (S10), with the number of open channels, which is determined solely by the dispersion relation given by Eq. (S1), is presented in Fig. 1.

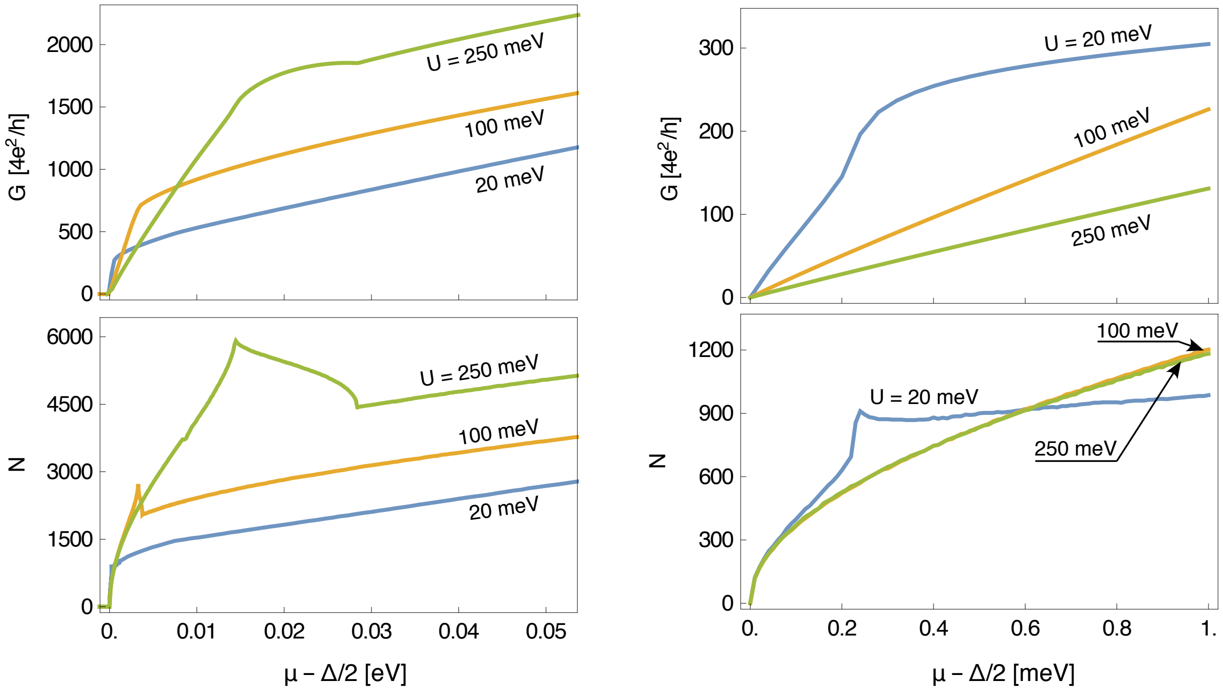


FIG. 1: The conductance (top) and the number of open channels (bottom) for an abrupt potential barrier in BLG, corresponding to the width $W = 10^3\, l_\perp = 1.77\,\mu$m and the trigonal-warping strength $t' = 0.3\,$eV, displayed as functions of the chemical potential. The electrostatic bias between the layers ($U$) is specified for each line. Right panels are zoom-ins, for low values of $\mu - \Delta/2$, for the data shown in left panels.

### B. Mode-matching for a rectangular sample

In order to determine the transmission probability at a given energy: $T(E)$, for a rectangular sample attached to the two heavily-doped regions (the *leads*), we employ the computational scheme similar to the presented in Ref. [3]. However, at finite-precision arithmetics, the mode-matching equations become ill-defined for sufficiently large $L$ and $\mu$, since they contain both exponentially-growing and exponentially-decaying coefficients. This difficulty can be overcome by dividing the sample area ($0 < x < L$) into $N_{\rm div}$ consecutive, equally-long parts, and then matching the wave functions for all ($N_{\rm div}$+1) interfaces. Typically, using the double-precision arithmetic, we put $N_{\rm div} = 20$ for $L = W/20 = 10^4\, l_\perp$. The necessary number of different transverse momenta $k_y = 2\pi q/W$ (where $q = 0, \pm 1, \pm 2, \dots, \pm q_{\rm max}$) varies with the energy $E$, scaling roughly as $2q_{\rm max} + 1 \propto \sqrt{|E| - \Delta/2}$ (for $|E| > \Delta/2$). For instance, to determine $T(E)$ with a 10-digit accuracy for $\Delta = U = 0$ we took: $1955 \leqslant 2q_{\rm max} + 1 \leqslant 8149$, with the lower (upper) value corresponding to $E = 0$ and $t' = 0.1\,$eV ($E = 2\,$meV and $t' = 0.35\,$eV).

## III. SIMPLIFIED MODELS FOR TRANSMISSION-ENERGY DEPENDENCE

### A. Basic definitions

For sufficiently large $\Delta$, transmission spectra $T(E)$ for either the single-barrier or the rectangular-sample case show essentially abrupt switching near $E \approx \Delta/2$, with some secondary details becoming irrelevant when calculating thermoelectric properties at nonzero temperature. Therefore, one can consider a family of simplified models for transmission-energy dependence, as given by Eq. (13) in the main text

$$T^{(\alpha)}(E) = \mathcal{C}^{(\alpha)}(\Delta) \times \begin{cases} \delta(E - \frac{1}{2}\Delta) + \delta(E + \frac{1}{2}\Delta) & \text{for } \alpha = 0 \\ \Theta(|E| - \frac{1}{2}\Delta)\left(|E| - \frac{1}{2}\Delta\right)^{\alpha - 1} & \text{for } \alpha > 0 \end{cases}, \tag{S11}$$

with $\delta(x)$ being the Dirac delta function, and $\Theta(x)$ being the Heaviside step function. A compact form of Eq. (S11) implies that the prefactor $\mathcal{C}^{(\alpha)}(\Delta)$ is dimensionless for $\alpha = 1$ only; in general, we have $\left[\mathcal{C}^{(\alpha)}(\Delta)\right] = {\rm eV}^{-\alpha+1}$ (for $\alpha \geqslant 0$).

The cummulants $L_n$, determining the thermoelectric properties via Eqs. (8)–(10) in the main text, are well-defined for the transmision-energy dependence of the form $T^{(\alpha)}(E)$ (S11) with arbitrary $\alpha \geqslant 0$. Substituting the derivative of the Fermi-Dirac distribution function

$$-\frac{\partial f_{\rm FD}}{\partial E} = \frac{1}{4\cosh^2\left[\,(E-\mu)/2k_BT\,\right]}\cdot\frac{1}{k_BT}, \tag{S12}$$

and introducing the dimensionless variables

$$t = \frac{E}{k_BT}, \qquad v = \frac{\mu}{k_BT}, \qquad u = \frac{\Delta}{2k_BT}, \tag{S13}$$

we can write

$$L_n^{(\alpha)} = \frac{g_sg_v}{h}\,\frac{(k_BT)^n}{4}\int dt\,(t-v)^n\,T^{(\alpha)}(t\cdot k_BT)\cosh^{-2}\left(\frac{t-v}{2}\right) \equiv \frac{g_sg_v}{h}(k_BT)^{n+\alpha-1}\,\mathcal{C}^{(\alpha)}(\Delta)\,\mathcal{L}_n^{(\alpha)}, \tag{S14}$$

where the last factor ($\mathcal{L}_n^{(\alpha)}$) is dimensionless and $\mathcal{C}$–independent. Explicitely, we obtain

$$\mathcal{L}_n^{(0)} = \frac{1}{4}(u-v)^n\cosh^{-2}\left(\frac{u-v}{2}\right) + \frac{1}{4}(-u-v)^n\cosh^{-2}\left(\frac{-u-v}{2}\right), \tag{S15}$$

$$\mathcal{L}_n^{(\alpha)} = \frac{1}{4}\int_y^{\infty} dt\,(t-v)^n(t-u)^{\alpha-1}\cosh^{-2}\left(\frac{t-v}{2}\right) + \frac{1}{4}\int_{-\infty}^{-y} dt\,(t-v)^n(-t-u)^{\alpha-1}\cosh^{-2}\left(\frac{t-v}{2}\right) \quad (\alpha>0). \tag{S16}$$

## B. Maximal absolute thermopower

Subsequent approximations, performed when calculating $\mathcal{L}_n^{(\alpha)}$ for $y \gg 1$, depend on mutual relation between $x$ and $y$. In particular, for the Seebeck coefficient, we first rewrite Eq. (9) from the main text as follows

$$S = \frac{k_B}{e}\,\mathcal{L}_1^{(\alpha)}\Big/\mathcal{L}_0^{(\alpha)}\,. \tag{S17}$$

Since the maximal $|S|$ is expected for $|v| \ll u$, we can employ the approximation

$$\frac{1}{4}\cosh^{-2}\left(\frac{t-v}{2}\right) \approx \begin{cases} e^{-t+v} & \text{for } u<t<\infty, \\ e^{t-v} & \text{for } -\infty<t<-u, \end{cases} \tag{S18}$$

(valid for $u \pm v \gg 1$), in order to get closed-form approximating expressions for the first three cumulants

$$\mathcal{L}_0^{(\alpha)} \approx e^{v-u} + e^{-v-u}, \tag{S19}$$

$$\mathcal{L}_1^{(\alpha)} \approx e^{v-u}(-v+u+\alpha) - e^{-v-u}(v+u+\alpha), \tag{S20}$$

$$\mathcal{L}_2^{(\alpha)} \approx e^{v-u}\left[(v-u)(v-u-2\alpha)+\alpha(\alpha+1)\right] + e^{-v-u}\left[(v+u)(v+u+2\alpha)+\alpha(\alpha+1)\right]. \tag{S21}$$

The right-hand side of Eq. (S17) can now be approximated by

$$S \approx \frac{k_B}{e}\,\left[\,(u+\alpha)\tanh v - v\,\right], \tag{S22}$$

with the maximal absolute value

$$|S|_{\max}\,(k_B/e)^{-1} \approx \sqrt{(u+\alpha)(u+\alpha-1)} - \ln\left(\sqrt{u+\alpha}+\sqrt{u+\alpha-1}\right), \tag{S23}$$

appearing for

$$v_{\max}^{|S|} \approx \pm\ln(\sqrt{u+\alpha-1}+\sqrt{u+\alpha}). \tag{S24}$$

These are Eqs. (14) and (15) in the main text.

### C. Thermoelectric figure of merit ($ZT$) for $T \to 0$

Similarly, neglecting the phononic part of the thermal conductivity (or, equivalently, taking the $T \to 0$ limit) we can express the thermoelectric figure of merit as follows

$$ZT(T \to 0) = ZT_{\text{el}} \equiv \frac{GS^2T}{K_{\text{el}}} = \frac{\left(\mathcal{L}_1^{(\alpha)}\right)^2}{\mathcal{L}_0^{(\alpha)}\mathcal{L}_2^{(\alpha)} - \left(\mathcal{L}_1^{(\alpha)}\right)^2}. \tag{S25}$$

This time, the approximation of Eqs. (S19)–(S21) does not lead to closed-form expressions for $ZT_{\text{el,max}}^{(\alpha)}$; least-square fitting of power-law formulas for $10 \leqslant u \leqslant 30$ brought us to

$$ZT_{\text{el, max}}^{(\alpha=1)} \approx 0.192(2) \cdot u^{2.374(3)}, \qquad ZT_{\text{el, max}}^{(\alpha=2)} \approx 0.1809(4) \cdot u^{2.217(1)}, \tag{S26}$$

with standard deviations for the last digit specified by numbers in parentheses. For $T > 0$, we generally have $ZT < ZT_{\text{el, max}}$, and the unlimited increase of $ZT$ with $u$ is not observed; however, we have $ZT \sim ZT_{\text{el, max}}^{(\alpha=1)}$ (up to the order of magnitude) for $T = 1\,\text{K}$ and $u \sim 1$.

### D. $ZT$ at finite temperatures and the power factor

In contrast with the $T \to 0$ limit discussed above, for any $T > 0$ there exists a value of $\Delta$, above which the electronic part of the thermal conductance is suppressed ($K_{\text{ph}} > K_{\text{el}}$). In turn, for $u \gg 1$ (being equivalent to $\Delta \gg k_BT > 0$), one can expect that the figure of merit

$$ZT(\Delta \gg k_BT > 0) \approx ZT_{\text{ph}} \equiv \frac{GS^2T}{K_{\text{ph}}} = \frac{T}{K_{\text{ph}}(T)}\,\frac{L_1^2}{T^2L_0}, \tag{S27}$$

where we have emphasised that the phononic part of thermal conductance depends only on temperature, $K_{\text{ph}} = K_{\text{ph}}(T)$. Subsequently, when looking for the maximal $ZT$ as a function of the chemical potential $\mu$ at a fixed $T$, one need to focus on the maximal power factor which is, for the transmission-energy dependence of the form $T^{(\alpha)}(E)$ (S11), given by

$$\left(GS^2\right)_{\text{max}}^{(\alpha)} = \frac{g_sg_v}{h}k_B^2(k_BT)^{\alpha-1}\,\mathcal{C}^{(\alpha)}(\Delta)\left[\left(\mathcal{L}_1^{(\alpha)}\right)^2\Big/\mathcal{L}_0^{(\alpha)}\right]_{\text{max}}. \tag{S28}$$

Defining $\mathcal{M}_{\text{max}}^{(\alpha)} = \left[\left(\mathcal{L}_1^{(\alpha)}\right)^2\Big/\mathcal{L}_0^{(\alpha)}\right]_{\text{max}}$, we restore the structure of Eq. (19) in the main text.

As the maximal $ZT$ corresponds to $v_{\text{max}}^{ZT} \sim u$, the approximating Eq. (S18) cannot be applied in this case. Instead, for $u \gg 1$ we have

$$\mathcal{L}_n^{(\alpha)} \equiv \mathcal{L}_{n,+}^{(\alpha)} + \mathcal{L}_{n,-}^{(\alpha)} \approx \mathcal{L}_{n,+}^{(\alpha)}, \tag{S29}$$

where the parts $\mathcal{L}_{n,+}^{(\alpha)}$ and $\mathcal{L}_{n,-}^{(\alpha)}$ are the integrals over $t > 0$ and $t < 0$ (respectively) in Eq. (S16). The results are

$$\mathcal{M}_{\text{max}}^{(\alpha=1)} \approx 1.265, \qquad \mathcal{M}_{\text{max}}^{(\alpha=2)} \approx 4.060, \tag{S30}$$

corresponding to

$$v_{\text{max}}^{ZT} \approx u - 1.145 \;\text{ for }\; \alpha = 1, \qquad \text{or} \qquad v_{\text{max}}^{ZT} \approx u + 0.668 \;\text{ for }\; \alpha = 2. \tag{S31}$$

The above Eqs. (S30) and (S31) are equivalent to Eqs. (16) and (17) in the main text.

## IV. PHONONIC PART OF THE THERMAL CONDUCTIVITY

### A. Brief overview

Here we overwiew the Callaway method [4], further modified by Alofi and Srivastava [5, 6] in order to determine the phononic part of the thermal conductance $K_{\text{ph}}$; see Eq. (12) in the main text. For the sake of consistency with

TABLE I: Parameters used in our numerical calculations. Most of the values are taken from Refs. [8, 9].

| Symbol | Numerical value | Units |
|---|---|---|
| $L$ | $1.77 \times 10^{-5}$ | m |
| $d$ | $3.3544 \times 10^{-10}$ | m |
| $V_m$ | $5.3 \times 10^{-6}$ | $\mathrm{m^3/mol}$ |
| $v_l$ | $2.16 \times 10^{4}$ | m/s |
| $v_t$ | $1.4 \times 10^{4}$ | m/s |
| $b$ | $3.13 \times 10^{-7}$ | $\mathrm{m^2/s}$ |
| $\zeta$ | $946091^a$ or $0^b$ | $\mathrm{m^2/s^2}$ |
| $B_N$ | $3.18 \times 10^{-25}$ | $\mathrm{s\,K^{-3}}$ |
| $B_U$ | $4.77 \times 10^{-25}$ | $\mathrm{s\,K^{-3}}$ |
| $\alpha$ | 3 | – |
| $A_d$ | 0.00169 | – |
| $\omega^D_{LA}$ | 472.6 | THz |
| $\omega^D_{TA}$ | 306.4 | THz |
| $\omega^D_{ZA}$ | 149.9 | THz |
| $\bar{\Theta}$ | 2365.4 | K |

[a]BLG; [b]MLG.

the notation of Refs. [5, 6], let us define the *thermal conductivity* for a rectangular BLG sample

$$\kappa_{\mathsf{el,ph}} = \frac{L}{2d}\frac{K_{\mathsf{el,ph}}}{W}, \tag{S32}$$

with $\mathsf{el}$ ($\mathsf{ph}$) denoting the electronic (phononic) part, $L$ and $W$ the sample length and width (respectively), and $d = 0.335\,\mathrm{nm}$ the separation between graphene layers. (For the remaining model parameters, see Table I.)

The phononic part of the thermal conductivity — in the remaining of this section simply denoted as $\kappa \equiv \kappa_{\mathsf{ph}}$ — can be calculated in the two steps, earlier presented in Ref. [6]:

*In the first step,* sufficient for the case of low temperatures, one can simply use the Debye approximation, in which a relevant element of the conductivity tensor reads

$$\kappa^D_{x,x} = \frac{\hbar^2 d}{2V_m k_B T^2}\sum_p \int_0^{\omega_{D,p}} d\omega\, \omega^2 v_p^2 \tau_p D_p(\omega)\, n(\omega)\,[n(\omega)+1]\,, \tag{S33}$$

where $V_m$ ($= 5.3 \times 10^{-6}\,\mathrm{m^3/mol}$) is the molar volume, $n(\omega)$ is the Bose-Einsten distribution function, $\omega_{D,p}$ is the Debye frequency (with the index $p$ labeling phonon polarization, $p = LA$, $TA$, or $ZA$; the corresponding phonon frequencies are listed in Table I). The relaxation time $\tau_p$, group velocity $v_p$ and density of states $D_p(\omega)$ are defined in next three subsections.

*The second step,* necessary at higher temperatures, requires one also to calculate a correction originating from the momentum conservation in the three-phonon processes of the type $N$. Such a correction reads

$$\kappa^{corr}_{x,x} = \frac{\hbar^2 d}{2V_m k_B T^2}\sum_p \frac{\left\{\int_0^{\omega_{D,p}} d\omega\, \omega^2 v_p^2 \tau_p \tau_N^{-1} D_p(\omega)\, n(\omega)\,[n(\omega)+1]\right\}^2}{\int_0^{\omega_{D,p}} d\omega\, \omega^2 v_p^2 \tau_p \tau_N^{-1}\left(1-\tau_p\tau_N^{-1}\right) D_p(\omega)\, n(\omega)\,[n(\omega)+1]}, \tag{S34}$$

where $\tau_N = B_N \omega^2 T^3$ (here $B_N = 3.18 \times 10^{-25}\,\mathrm{s\,K^{-3}}$ is a parameter fitted to the experimental data) denotes the relaxation time for three-phonon processes of the type $N$. The prefactor 1/2, in both $\kappa^D_{x,x}$ and $\kappa^{corr}_{x,x}$, originates from averaging the group velocity over possible directions (we focus here on the in-plane heat transfer, see Ref. [7]).

### B. Relaxation times

We take into account the three main sources of the phonon scattering: boundaries (index $bs$), point defects and isotopes ($pd$), and three-phonon scattering processes ($anh$). Assuming that these mechanisms are mutually independent,

we employ the Matthiessen rule to write down the formula for the total relaxation time $\tau_p$:

$$\tau_p^{-1} = \tau_{p,\,bs}^{-1} + \tau_{p,\,pd}^{-1} + \tau_{p,\,anh}^{-1}. \tag{S35}$$

The elements on the right-hand side of Eq. (S35) are given by:

$$\tau_{p,\,bs}^{-1} = v_p/L,$$

where $L$ is the length of the system [8], $v_p$ is the group velocity for phonons of the polarization $p$,

$$\tau_{p,\,pd}^{-1} = \frac{2\pi}{\omega_{D,p}^2}\omega^3 A_d,$$

where $\omega_{D,p}$ is the Debye frequency for the polarization $p$, $A_d$ is a parameter quantifying the concentration of impurities (i.e., point defects or $C^{13}$ atoms), and

$$\tau_{p,\,anh}^{-1} = \left\{B_N + B_U \exp\left[-\bar{\Theta}/\left(\alpha T\right)\right]\right\}\omega^2 T^3,$$

with the parameters $B_U = 4.77\times10^{-25}\,\mathrm{s\,K^{-3}}$ and $B_N = 3.18\times10^{-25}\,\mathrm{s\,K^{-3}}$ (adjusted to match the results of Ref. [5]), $\alpha = 3$, and $\bar{\Theta} = 2365.4\,\mathrm{K}$ being the Debye temperature averaged over the polarizations $p = LA$, $TA$, $ZA$.

### C. Group velocities

The group velocity $v_p$ is defined as a derivative of the frequency $\omega_p$ over the wave vector $q$,

$$v_p = \frac{\partial\omega_p}{\partial q}. \tag{S36}$$

In the case of monolayer graphene, group velocities for acoustic phonons are given by

$$v_{LA}^{MLG} = v_l, \tag{S37}$$
$$v_{TA,}^{MLG} = v_t, \tag{S38}$$
$$v_{ZA}^{MLG} = 2\sqrt{b\omega_{ZA}}, \tag{S39}$$

where $v_l = 2.16\times10^4$ m/s, $v_t = 1.4\times10^4$ m/s, and $b = 3.13\times10^{-7}\,\mathrm{m^2/s}$. In the case of bilayer graphene, it becomes necessary to take the coupling between the layers into account. This alters only the expression for $v_{ZA}$, leading to

$$v_{LA}^{BLG} = v_l, \tag{S40}$$
$$v_{TA}^{BLG} = v_t, \tag{S41}$$
$$v_{ZA}^{BLG} = \gamma\sqrt{\gamma-\zeta}\left(\sqrt{2}\,\omega_{ZA}b\right)^{-1}, \tag{S42}$$

where $\gamma = \sqrt{\zeta^2 + (2b\omega)^2}$, and $\zeta = 946091\,\mathrm{m^2/s}$ is a parameter quantifying the coupling between the layers. Taking the $\zeta \to 0$ limit, we obtain the expression for decoupled layers. In such a case, group velocities for monolayer (MLG) and bilayer graphene (BLG) are the same.

### D. Phononic density of states

In the case of $LA$ or $TA$ polarization, the density of states (DOS) reads

$$D_p(\omega) = \begin{cases} \arcsin\left(\omega/\omega_z\right)\left(V_m/d\right)\omega/\left(\pi v_p\right)^2, & \text{if}\, \omega \le \omega_z, \\ \left(V_m/d\right)\omega/\left(2\pi v_p^2\right), & \text{if}\, \omega > \omega_z, \end{cases} \tag{S43}$$

where $\omega_z = 5.8\,\mathrm{THz}$ for BLG (or $\omega_z = 0$ for MLG). In the case of $ZA$ polarization, we have

$$D_{ZA}(\omega) = \begin{cases} \left(V_m/d\right)\omega/\left(2\pi^2 b\omega_z'\right)\int_0^{\arcsin(2b\omega/\gamma)}\left\{1-\left[\gamma\sin\left(\phi\right)/\left(2b\omega_z'\right)\right]^2\right\}^{-1/2} d\phi, & \text{if }\, \omega \le \omega_z', \\ \left(V_m/d\right)\omega/\left(\pi^2\gamma\right)\int_0^{\pi/2}\left\{1-\left[2b\omega_z'\sin\left(\phi\right)/\gamma\right]^2\right\}^{-1/2} d\phi, & \text{if}\, \omega > \omega_z', \end{cases} \tag{S44}$$

where $\omega_z' = 14.48\,\mathrm{THz}$ for BLG (or $\omega_z' = 0$ for MLG).

### E. An abrupt interface

In the limit of $L \to 0$, our model of thermal conductivity is noticeably simplified: The three-phonon scattering processes, as well as the contributions from impurities and boundaries, become irrelevant (namely, we can put $\tau_p^{-1} \to \tau_{p,\,bs}^{-1}$, $\tau_{p,\,pd}^{-1} \to 0$, and $\tau_{p,\,anh}^{-1} \to 0$ in Eq. (S35)). In turn, Eq. (S33) simplifies to

$$\kappa_{x,x}^{0} = \frac{\hbar^2 L d}{2 V_m k_B T^2} \sum_p \int_0^{\omega_p^D} d\omega \omega^2 v_p D_p(\omega)\, n(\omega) \left[ n(\omega) + 1 \right], \tag{S45}$$

showing an explicit linear dependence of the thermal conductivity on the length $L$, and leading to a finite thermal conductance per unit width, $K_{\mathsf{ph}}/W = (2d/L)\kappa_{x,x}^0$ [see also Eq. (S32)].

---

[1] E. McCann and V.I. Fal'ko, Phys. Rev. Lett. **96**, 086805 (2006); E. McCann, Phys. Rev. B **74**, 161403(R) (2006).
[2] E. McCann and M. Koshino, Rep. Prog. Phys. **76**, 056503 (2013).
[3] G. Rut and A. Rycerz, Europhys. Lett. **107**, 47005 (2014).
[4] J. Callaway, Phys. Rev. **113**, 1046 (1959).
[5] A. Alofi and G.P. Srivastava, Phys. Rev. B **87**, 115421 (2013); A. Alofi and G.P. Srivastava, Appl. Phys. Lett. **104**, 031903 (2014).
[6] A. Alofi, *Theory of Phonon Thermal Transport in Graphene and Graphite*, Ph.D. Thesis, University of Exeter, 2014; http://hdl.handle.net/10871/15687.
[7] P.G. Klemens, Thermal Conductivity **22**, 365–365 (1993).
[8] J. Callaway, *Quantum theory of the solid state*, Academic Press, San Diego, 2013.
[9] T. Nihira and T. Iwata, Phys. Rev. B **68**, 134305 (2005).
